# Supplementary material for: OptEmbed: Learning Optimal Embedding Table for Click-through Rate Prediction
Source: arXiv:2208.04482 source file (2022-09-06)
Supplement: Supplementary file 1 [file reproduce.tex]

\section{Reproducibility} \label{appendix:reproduce}

\setcounter{table}{0}

\subsection{Source Code}
The source code of our \textit{OptEmbedding} method is available here\footnote{https://github.com/fuyuanlyu/OptEmbed}. Our implementation is based on a public Pytorch library for CTR prediction\footnote{https://github.com/rixwew/pytorch-fm}. For other comparison methods, we reuse the official implementation for the PEP\footnote{https://github.com/ssui-liu/learnable-embed-sizes-for-RecSys}\cite{PEP} and QR\footnote{https://github.com/facebookresearch/dlrm}\cite{QR} methods. Due to the lack of available implementation for the AutoDim\cite{AutoDim} and AutoField\cite{autofield} method, we re-implement them based on the details provided by the authors.

\subsection{Hyper-parameter settings}
Here we list all the hyper-parameters we used in the supernet training stage for each model in Table \ref{Table:param}. The following procedure describes how we determine these hyper-parameters. 

First, we determine the hyper-parameters of the basic models by grid search: learning ratio and $l_2$ regularization. We select the optimal learning ratio from \{1e-3, 3e-4, 1e-4, 3e-5, 1e-5\} and $l_2$ regularization from \{1e-3, 3e-4, 1e-4, 3e-5, 1e-5, 3e-6, 1e-6\}. Following previous work~\cite{IPNN}, Adam optimizer and Xavier initialization~\cite{Xavier} are adopted. Xavier initialises the weights in the model such that their values are subjected to a uniform distribution between $[-\sqrt{6/(n_{in}+n_{out})}$, $ \sqrt{6/(n_{in}+n_{out})}]$ with $n_{in}$ and $n_{out}$ being the input and output sizes of a hidden layer. Such initialization has been proven to be able to stabilize activations and gradients in the early stage of training~\cite{IPNN}. Batch normalization\cite{BatchNorm} has been applied to each fully-connected layer to avoid the internal covariate shift.

Second, we tune the hyper-parameters introduced by the \textit{OptEmbedding} method: learning ratio for threshold $\text{lr}^\text{t}$, threshold learning ratio decay $\gamma$, threshold regularization $\alpha$. We select the optimal threshold learning ratio $\text{lr}^\text{t}$ from \{1e-2, 1e-3, 1e-4\} and threshold regularization $\alpha$ from \{1e-4, 3e-5, 1e-5, 3e-6, 1e-6\}. During tuning process, we fix the optimal learning ratio and $l_2$ regularization determined in the first step. We select the optimal hyper-parameters based on the performance of supernet on validation set.

\begin{table}[tb]
    
	\centering
	\caption{Parameter Setup}
	\begin{tabular}{|c|c|c|c|}
	\hline
	    Params & Criteo & Avazu & KDD12 \\
	\hline
	    \multirow{2}{*}{General} 
	        & \multicolumn{3}{c|}{bs=2048, dim=64, opt=Adam} \\
	        & \multicolumn{3}{c|}{net=[1024, 512, 256], BN=True} \\
	\hline
	    \multirow{2}{*}{DeepFM} 
	        & lr=3e-5, $\text{l}_2$=1e-3 & lr=3e-4, $\text{l}_2$=1e-5 & lr=3e-5, $\text{l}_2$=1e-5 \\
	        & $\text{lr}^\text{t}$=1e-4, $\alpha$=1e-4 & $\text{lr}^\text{t}$=1e-4, $\alpha$=1e-6 & $\text{lr}^\text{t}$=1e-4, $\alpha$=1e-5 \\
	\hline
	    \multirow{2}{*}{DCN} 
	        & lr=3e-4, $\text{l}_2$=1e-5 & lr=1e-4, $\text{l}_2$=3e-5 & lr=1e-5, $\text{l}_2$=1e-6 \\
	        & $\text{lr}^\text{t}$=1e-4, $\alpha$=1e-5 & $\text{lr}^\text{t}$=1e-4, $\alpha$=1e-4 & $\text{lr}^\text{t}$=1e-4, $\alpha$=1e-5 \\
	\hline
	    \multirow{2}{*}{FNN}
	        & lr=3e-4, $\text{l}_2$=1e-5 & lr=1e-4, $\text{l}_2$=3e-5 & lr=1e-5, $\text{l}_2$=1e-6 \\
	        & $\text{lr}^\text{t}$=1e-4, $\alpha$=1e-5 & $\text{lr}^\text{t}$=1e-4, $\alpha$=1e-4 & $\text{lr}^\text{t}$=1e-4, $\alpha$=1e-5 \\
	\hline
	    \multirow{2}{*}{IPNN}
	        & lr=3e-4, $\text{l}_2$=1e-5 & lr=1e-4, $\text{l}_2$=3e-5 & lr=1e-5, $\text{l}_2$=1e-6 \\
	        & $\text{lr}^\text{t}$=3e-5, $\alpha$=1e-6 & $\text{lr}^\text{t}$=1e-4, $\alpha$=1e-4 & $\text{lr}^\text{t}$=1e-4, $\alpha$=1e-5 \\
	\hline
	\end{tabular}
	\begin{tablenotes}
    \footnotesize
    \item[1] Note: bs = batch size, opt=optimizer, net = MLP structure, BN = batch normalization, lr = learning rate on basic CTR model, dim = embedding dimension size, $\text{l}_2$ = $\text{l}_2$ regularization on basic CTR model, $\text{lr}^\text{t}$ = learning ratio on threshold, $\alpha$ = threshold regularization term.
    \end{tablenotes}
	\label{Table:param}
\end{table}

Additionally, for the evolutionary search stage, we adopt the same hyper-parameters from previous work\cite{One-shot}. For all experiments, mutation number $n_m = 10$, crossover number $n_c = 10$, max iteration $T=30$, mutation probability $prob = 0.1$ and $k=15$.

Finally, for the retraining stage, we adopt the same learning rate and weight decay from Table \ref{Table:param}.
